# Supplementary material for: Graph Pricing Problem on Bounded Treewidth, Bounded Genus and k-partite graphs
Source: arXiv:1203.1940 source file (2013-11-12)
Supplement: Supplementary file 1 [file prelim_appendix.tex]

%\section{Proof of Lemma~\ref{lemma: poly budget}}\label{sec:poly_budget_proof}
%
%Let $B_{\max}$ denote the maximum budget among all consumers, and $M= \epsilon B_{\max}/nm$. Notice that $B_{\max} \leq \opt$. We create a new instance of the problem as follows: For each consumer $u v\in E$, we define new budget $B'_{e} = \floor{B_e/M}$. Let $p^*$ be the optimal price for the old instance. We define the price $p'(v) = \floor{p^*(v)/M}$.
%
%First it is clear that the first property holds because $B_e/M \leq O(mn/\epsilon)$. To prove the second property, let $\opt'$ denote the optimal revenue of the new instance. Clearly, $M \opt' \leq \opt$, since any price of new instance can be turned into price of the old instance that collects $M$ times as much. Next, for any consumer $e=uv$ that collects revenue $p^*(u)+p^*(v)$ in the old instance, we have $p'(u) + p'(v) \leq \floor{(p^*(u) + p^*(v))/M}\leq B'_e$, so this consumer does not go over budget with price $p'$ in the new instance. And $\sum_{e\in E} M r'(e) \geq \sum_{e \in E} \left( r(e) - 2M \right) \geq (1-\epsilon) \opt \geq (1-\epsilon) M\opt'$. Therefore, the revenue collected by $p'$ is at least $(1-\epsilon)\opt'$.
%
%Observe that any $\alpha$-approximation algorithm for the new instance can be turned into $(1+2\epsilon)\alpha$ approximation algorithm for the old instance as follows: Let $p'$ be the price that collects a total revenue of $\opt'/\alpha$ in the new instance. We define $p(v) = M p'(v)$ for all $v \in V$. Then the total revenue we get is $\frac{M \opt'}{\alpha} \geq \frac{(1-\epsilon)\opt}{\alpha} \geq \frac{\opt}{(1+2\epsilon)\alpha}$.
%
